# Supplementary material for: Artificial social influence via human-embodied AI agent interaction in immersive virtual reality (VR): Effects of similarity-matching during health conversations
Source: arXiv:2406.05486 ancillary file (2024-09-12)
Supplement: Supplementary file 1 [file Appendix__V2.pdf]

## Appendix

### A1. Effect of Gender Matching on Additional Evaluations of the VR-ECAs

We examined the effect of gender matching on how participants evaluated the embodied agents (beyond likeability) by fitting a series of linear models, with agent and user gender as the main and interaction effects. Overall, female participants tended to evaluate the agents more positively, and the differences between gender pairings were greater for male agents vs. female agents (see Figure A1 and Table A1).

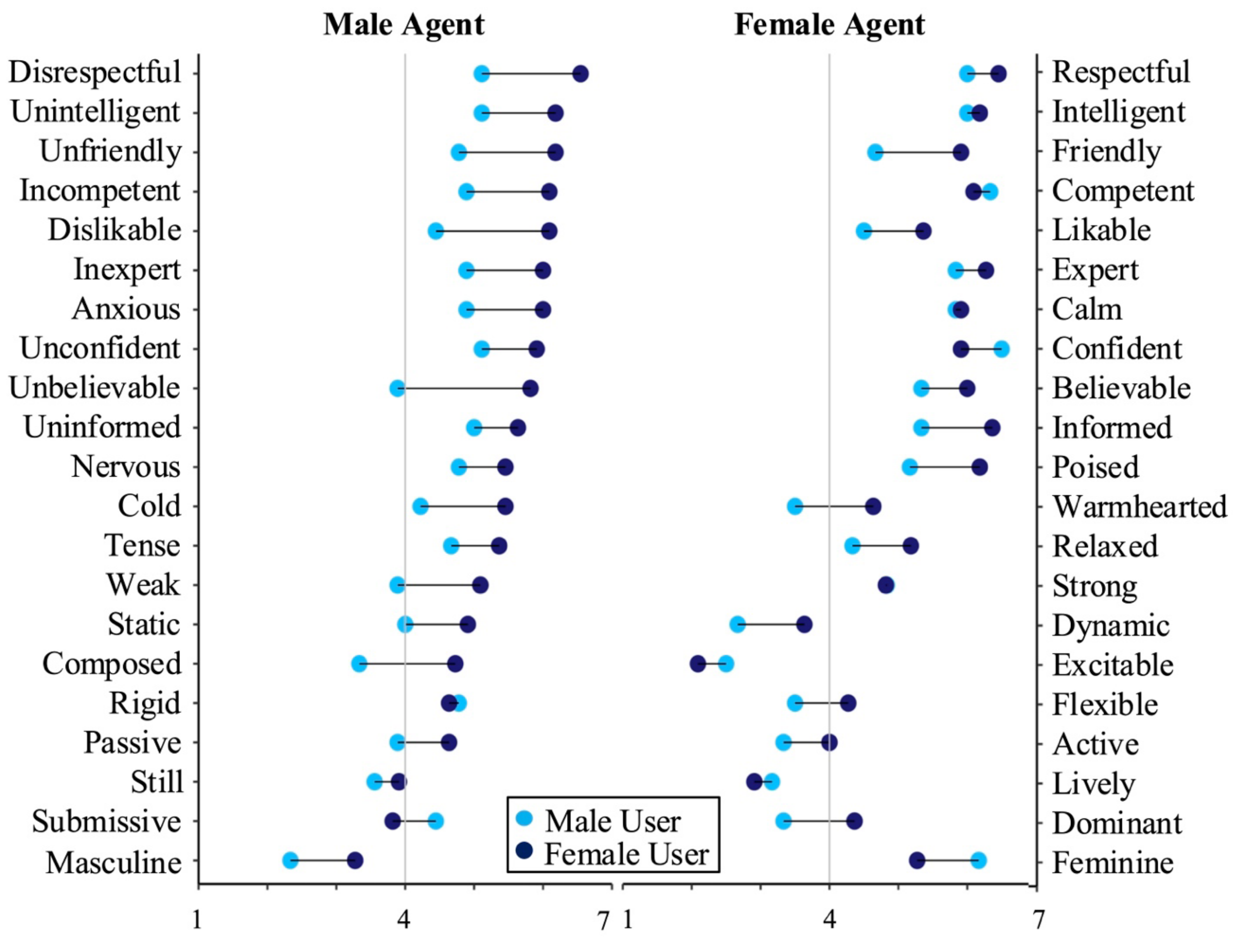


Figure A1. Evaluation of VR-ECAs by Agent and User Gender Pairings.

Table A1. Effect of VR-ECA and User Gender Pairings on Agent Evaluation

| | *Estimate* | *S.E.* | *t* | *p-value* |
|---|---|---|---|---|
| ***Unbelievable (1) - Believable (7)*** | | | | |
| Intercept | 3.89 | .46 | *8.39* | **<.001** |
| VR-ECA Gender: Female (vs. Male) | 1.44 | .73 | *1.97* | .057 |
| User Gender: Female (vs. Male) | 1.94 | .61 | *3.17* | **.0033** |
| VR-ECA Gender: Female x User Gender: Female | -1.28 | .94 | *-1.35* | .19 |
| ***Unlikable (1) - Likable (7)*** | | | | |
| Intercept | 4.44 | .40 | *11.20* | **<.001** |
| VR-ECA Gender: Female (vs. Male) | .056 | .62 | *.089* | .93 |
| User Gender: Female (vs. Male) | 1.64 | .52 | *3.12* | **.0037** |
| VR-ECA Gender: Female x User Gender: Female | -.84 | .81 | *-1.04* | .31 |
| ***Disrespectful (1) - Respectful (7)*** | | | | |
| Intercept | 2.89 | .38 | *7.65* | **<.001** |
| VR-ECA Gender: Female (vs. Male) | -.89 | .60 | *-1.49* | .15 |
| User Gender: Female (vs. Male) | -1.39 | .50 | *-2.78* | **.0089** |
| VR-ECA Gender: Female x User Gender: Female | .89 | .77 | *1.16* | .26 |
| ***Unfriendly (1) - Friendly (7)*** | | | | |
| Intercept | 4.78 | .43 | *11.06* | **<.001** |
| VR-ECA Gender: Female (vs. Male) | -.11 | .68 | *-.16* | .87 |
| User Gender: Female (vs. Male) | 1.39 | .57 | *2.43* | **.021** |
| VR-ECA Gender: Female x User Gender: Female | -.16 | .88 | *-.18* | .86 |
| ***Unexcitable (1) - Excitable (7)*** | | | | |
| Intercept | 3.33 | .50 | *6.62* | **<.001** |
| VR-ECA Gender: Female (vs. Male) | -.83 | .80 | *-1.05* | .30 |
| User Gender: Female (vs. Male) | 1.42 | .67 | *2.13* | **.041** |
| VR-ECA Gender: Female x User Gender: Female | -2.12 | 1.03 | *-2.06* | **.047** |
| ***Cold (1) - Warmhearted (7)*** | | | | |
| Intercept | 4.22 | .45 | *9.37* | **<.001** |
| VR-ECA Gender: Female (vs. Male) | -.72 | .71 | *-1.01* | .32 |
| User Gender: Female (vs. Male) | 1.19 | .60 | *2.00* | .054 |
| VR-ECA Gender: Female x User Gender: Female | -.094 | .92 | *-.10* | .92 |

| | | | | |
|---|---|---|---|---|
| ***Weak (1) - Strong (7)*** | | | | |
| Intercept | 3.89 | .43 | *9.00* | **<.001** |
| VR-ECA Gender: Female (vs. Male) | .94 | .68 | *1.38* | .18 |
| User Gender: Female (vs. Male) | 1.28 | .57 | *2.24* | **.032** |
| VR-ECA Gender: Female x User Gender: Female | -1.41 | .88 | *-1.60* | .12 |
| ***Incompetent (1) - Competent (7)*** | | | | |
| Intercept | 4.89 | .32 | *15.37* | **<.001** |
| VR-ECA Gender: Female (vs. Male) | 1.44 | .50 | *2.87* | **.0071** |
| User Gender: Female (vs. Male) | 1.20 | .42 | *2.84* | **.0077** |
| VR-ECA Gender: Female x User Gender: Female | -1.43 | .65 | *-2.20* | **.035** |
| ***Anxious (1) - Calm (7)*** | | | | |
| Intercept | 4.89 | .34 | *14.23* | **<.001** |
| VR-ECA Gender: Female (vs. Male) | .94 | .54 | *1.74* | .091 |
| User Gender: Female (vs. Male) | 1.03 | .45 | *2.26* | **.030** |
| VR-ECA Gender: Female x User Gender: Female | -.46 | .70 | *-.66* | .51 |
| ***Inexpert (1) - Expert (7)*** | | | | |
| Intercept | 4.89 | .37 | *13.22* | **<.001** |
| VR-ECA Gender: Female (vs. Male) | .94 | .58 | *1.62* | .12 |
| User Gender: Female (vs. Male) | 1.11 | .49 | *2.27* | **.030** |
| VR-ECA Gender: Female x User Gender: Female | -1.04 | .75 | *-1.39* | .18 |
| ***Unintelligent (1) - Intelligent (7)*** | | | | |
| Intercept | 5.11 | .36 | *14.26* | **<.001** |
| VR-ECA Gender: Female (vs. Male) | .89 | .57 | *1.57* | .13 |
| User Gender: Female (vs. Male) | 1.06 | .47 | *2.23* | **.033** |
| VR-ECA Gender: Female x User Gender: Female | -.86 | .73 | *-1.17* | .25 |
| ***Masculine (1) - Feminine (7)*** | | | | |
| Intercept | 2.33 | .52 | *4.47* | **<.001** |
| VR-ECA Gender: Female (vs. Male) | 3.83 | .83 | *4.65* | **<.001** |
| User Gender: Female (vs. Male) | .83 | .69 | *1.21* | .24 |
| VR-ECA Gender: Female x User Gender: Female | -1.40 | 1.06 | *-1.32* | .20 |

| | | | | |
|---|---|---|---|---|
| ***Static (1) - Dynamic (7)*** | | | | |
| Intercept | 4.00 | .63 | *6.38* | **<.001** |
| VR-ECA Gender: Female (vs. Male) | -1.33 | .99 | *-1.35* | .19 |
| User Gender: Female (vs. Male) | .92 | .83 | *1.11* | .29 |
| VR-ECA Gender: Female x User Gender: Female | -.083 | 1.28 | -.065 | .95 |
| ***Unconfident (1) - Confident (7)*** | | | | |
| Intercept | 5.11 | .33 | *15.52* | **<.001** |
| VR-ECA Gender: Female (vs. Male) | 1.39 | .52 | *2.67* | **.012** |
| User Gender: Female (vs. Male) | .81 | .44 | *1.85* | .073 |
| VR-ECA Gender: Female x User Gender: Female | -1.41 | .67 | *-2.10* | **.044** |
| ***Rigid (1) - Flexible (7)*** | | | | |
| Intercept | 3.89 | .64 | *6.07* | **<.001** |
| VR-ECA Gender: Female (vs. Male) | -.56 | 1.02 | *-.55* | .59 |
| User Gender: Female (vs. Male) | .78 | .85 | *.92* | .37 |
| VR-ECA Gender: Female x User Gender: Female | -.21 | 1.30 | *-.16* | .87 |
| ***Tense (1) - Relaxed (7)*** | | | | |
| Intercept | 4.67 | .60 | *7.76* | **<.001** |
| VR-ECA Gender: Female (vs. Male) | -.33 | .95 | *-.35* | .73 |
| User Gender: Female (vs. Male) | .50 | .80 | *.63* | .53 |
| VR-ECA Gender: Female x User Gender: Female | .57 | 1.23 | *.46* | .65 |
| ***Nervous (1) - Poised (7)*** | | | | |
| Intercept | 4.78 | .40 | *11.96* | **<.001** |
| VR-ECA Gender: Female (vs. Male) | .39 | .64 | *.62* | .54 |
| User Gender: Female (vs. Male) | .64 | .53 | *1.21* | .24 |
| VR-ECA Gender: Female x User Gender: Female | .49 | .81 | *.61* | .55 |
| ***Uninformed (1) - Informed (7)*** | | | | |
| Intercept | 5.00 | .44 | *11.28* | **<.001** |
| VR-ECA Gender: Female (vs. Male) | .33 | .70 | *.48* | .64 |
| User Gender: Female (vs. Male) | .67 | .59 | *1.14* | .26 |
| VR-ECA Gender: Female x User Gender: Female | .40 | .90 | *.44* | .66 |

| | | | | |
|---|---|---|---|---|
| ***Submissive (1) - Dominant (7)*** | | | | |
| Intercept | 4.44 | .40 | *11.10* | **<.001** |
| VR-ECA Gender: Female (vs. Male) | -1.11 | .63 | *-1.76* | .089 |
| User Gender: Female (vs. Male) | -.61 | .53 | *-1.15* | .26 |
| VR-ECA Gender: Female x User Gender: Female | 1.68 | .82 | *2.06* | **.048** |
| ***Still (1) - Lively (7)*** | | | | |
| Intercept | 3.56 | .69 | *5.16* | **<.001** |
| VR-ECA Gender: Female (vs. Male) | -.39 | 1.09 | *-.36* | .72 |
| User Gender: Female (vs. Male) | .44 | .91 | *.49* | .63 |
| VR-ECA Gender: Female x User Gender: Female | -.91 | 1.40 | *-.65* | .52 |
| ***Passive (1) - Active (7)*** | | | | |
| Intercept | 4.78 | .59 | *8.14* | **<.001** |
| VR-ECA Gender: Female (vs. Male) | -1.28 | .93 | *-1.38* | .18 |
| User Gender: Female (vs. Male) | -.28 | .78 | *-.36* | .72 |
| VR-ECA Gender: Female x User Gender: Female | 1.18 | 1.20 | *.98* | .33 |

*Note. S.E. = Standard Error*
